# Supplementary material for: Large-eddy simulations of the flow around a NACA0012 airfoil at different angles of attack
Source: arXiv:1807.01576 source file (2018-07-04)
Supplement: Supplementary file 1 [file appendix.tex]

\appendix
% use \input for the appendix
\chapter{Appendix 1}\label{appendix_1}
\input{appendix/appendix_1}

\chapter{Appendix 2}\label{appendix_2}
\input{appendix/appendix_2}
